# Supplementary material for: Visual Captioning at Will: Describing Images and Videos Guided by a Few Stylized Sentences
Source: arXiv:2307.16399 source file (2023-07-31)
Supplement: Supplementary file 1 [file appendix.tex]

\newpage
\section{Appendix}
\subsection{Data Processing}
Following \cite{li2018delete} and \cite{riley2020textsettr}, we utilize the code shown in Figure \ref{fig:codes} to process each sample in our training corpus and convert it to a standard format. In this work, we set the maximum sentence length to $32$ tokens and filter out samples that exceed this length.
\begin{figure}[h]
    \centering
    \includegraphics[width=\linewidth]{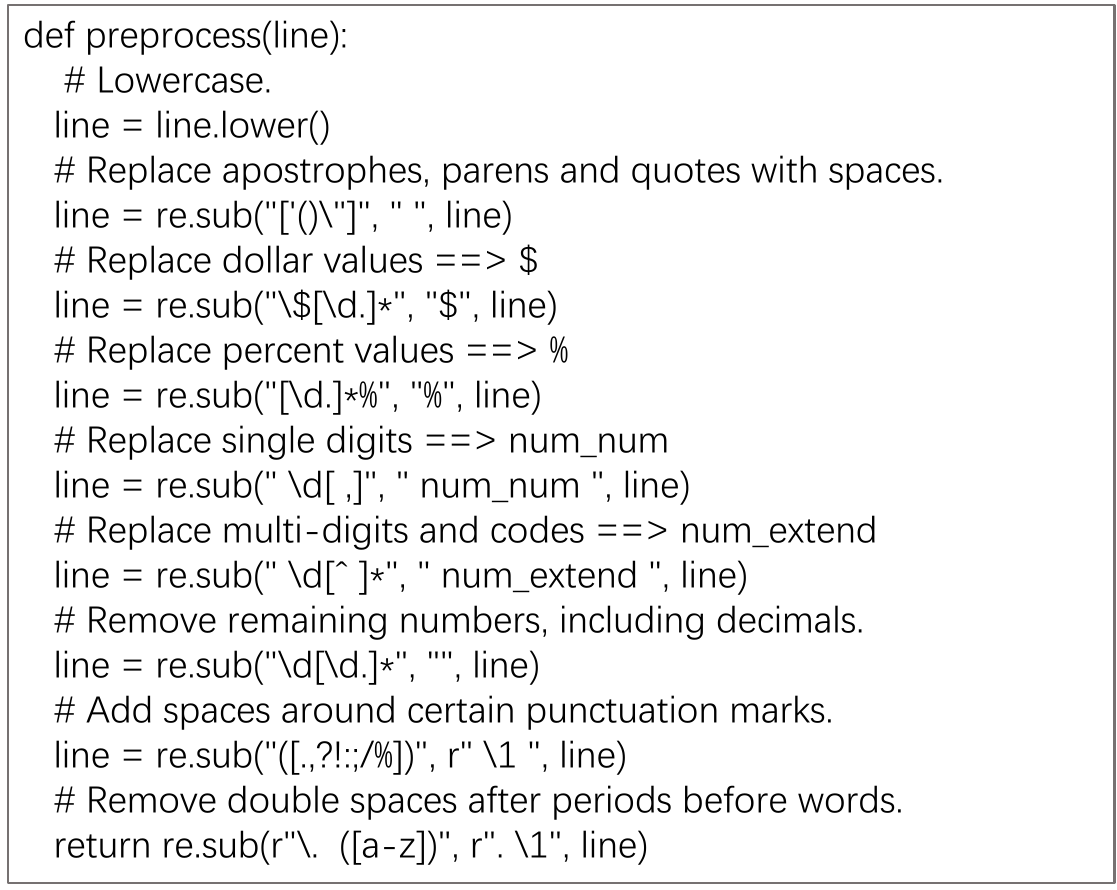}
    \caption{Codes}
    \label{fig:codes}
\end{figure}
\subsection{Perplexity}

Following previous works \cite{tan2022detach,guo2019mscap}, we present the perplexity scores of proposed FS-StyleCap and other baselines as a proxy for fluency. As shown in Table \ref{table:ppl}, our few-shot results outperform the full methods StyleNet \cite{gan2017stylenet} and MSCap \cite{guo2019mscap}. However, there is still a small gap between our few-shot approach and the best fully trained model CapDec \cite{nukrai2022capdec}. We find that because FS-StyleCap is not trained on SentiCap, it might generate some expressions that do not exist in SentiCap, leading to higher perplexity scores for these results.
%Due to a domain gap between SentiCap and our training corpus, we evaluate two perplexity scores. The first was calculated by SRILM \cite{stolcke2002srilm} on SentiCap, while the second was calculated by SRILM on our corpus. For the latter, we split all the personality traits into positive and negative types to create the training corpus for SRILM. 
However, it is worth noting that prior work has demonstrated perplexity to be a poor measure of fluency. 

\begin{table}[h]
\centering
\caption{Perplexity scores.}
\label{table:ppl} 
\fontsize{8}{14}\selectfont
\begin{tabular}{cccccc}
\toprule
\multicolumn{2}{c}{} & \multicolumn{2}{c}{\textbf{Positive}} & \multicolumn{2}{c}{\textbf{Negative}} \\
\cline{3-6} 
 & \textbf{Model} & \textbf{Data} & \textbf{PPL$\downarrow$} & \textbf{Data} & \textbf{PPL$\downarrow$} \\
 \midrule
\multirow{3}{*}{\textbf{Few-Shot}} & \multicolumn{1}{c|}{FS-StyleCap} & \multicolumn{1}{c|}{1} & \multicolumn{1}{c|}{18.3} & \multicolumn{1}{c|}{1} & 16.5 \\
 & \multicolumn{1}{c|}{FS-StyleCap} & \multicolumn{1}{c|}{5} & \multicolumn{1}{c|}{19.4} & \multicolumn{1}{c|}{5} & 17.0 \\
 & \multicolumn{1}{c|}{FS-StyleCap} & \multicolumn{1}{c|}{100} & \multicolumn{1}{c|}{18.1} & \multicolumn{1}{c|}{100} & 17.5 \\
 \bottomrule
 \toprule
\multirow{3}{*}{\textbf{Full}} & \multicolumn{1}{c|}{StyleNet \cite{gan2017stylenet}} & \multicolumn{1}{c|}{2,994} & \multicolumn{1}{c|}{24.8} & \multicolumn{1}{c|}{2,991} & 25.0 \\
 & \multicolumn{1}{c|}{MSCap \cite{guo2019mscap}} & \multicolumn{1}{c|}{2,994} & \multicolumn{1}{c|}{19.6} & \multicolumn{1}{c|}{2,991} & 19.2 \\
 & \multicolumn{1}{c|}{CapDec \cite{nukrai2022capdec}} & \multicolumn{1}{c|}{2,994} & \multicolumn{1}{c|}{14.3} & \multicolumn{1}{c|}{2,991} & 13.1\\
 \bottomrule
\end{tabular}
\end{table}
\subsection{Stylized Samples}
In Table \ref{table:stylized_samples}, we show the examples which are used to guide our stylized generation.
\begin{table}[t]
\caption{The example sentences to guide the generation of different styles.}
\label{table:stylized_samples} 
\fontsize{5}{12}\selectfont
\begin{tabular}{cl}
\toprule
\textbf{Styles} & \multicolumn{1}{c}{\textbf{Samples}} \\
\midrule
\textbf{Positive} & \begin{tabular}[c]{@{}l@{}}1. A good man sitting at a relaxing hotel. \\ 2. A pretty woman sporting a cute dress.\\ 3. A happy cat that is laying down on a comfortable sofa.\\ 4. A great room with beautiful orange walls and relaxing chair.\\ 5. An interesting plant of broccoli growing inside of a fenced garden.\end{tabular} \\
\midrule
\textbf{Negative} & \begin{tabular}[c]{@{}l@{}}1. A bad boy riding a bad skateboard down the side walk. \\ 2. An abused woman works on her broken computer.\\ 3. A crazy cat laying down in dead leaves. \\ 4. A gloomy room filled with old furniture and an ugly wall. \\ 5. A broken tree and dead grass.\end{tabular} \\
\end{tabular}
\end{table}

\begin{table}[t]
\caption{The example sentences to guide the generation of different styles.}
\label{table:2} 
\fontsize{5}{12}\selectfont
\begin{tabular}{cl}
\toprule
\textbf{Styles} & \multicolumn{1}{c}{\textbf{Samples}} \\
\midrule
\textbf{Romantic} & \begin{tabular}[c]{@{}l@{}}1. This man makes me feel so much love. \\ 2. I love this dog couple playing in the snow!\\ 3. I love this dog couple playing in the snow!  \\ 4. I think this man is sweet, wish to pluck this for a special someone. \\ 5. A young boy is dancing around, enjoying time with his family.\end{tabular} \\
%\midrule
%\textbf{Adventurous} & \begin{tabular}[c]{@{}l@{}}1. I would try it! this house makes you want to go in and explore.  \\ 2. What a great day to discover some new plants! I love to see new places .\\ 3. I would love to go out on a nature hike and get close to animals like this.  \\ 4. They are having fun! Looks as if they are about to go to a football game. \\ 5. Sunsets like these are what makes me chase my next adventure.\end{tabular} \\
%\midrule
%\textbf{Memorable} & \begin{tabular}[c]{@{}l@{}}1. This reminds me of my mom .  \\ 2. I remember the childhood days of waking to the sounds of birds in summer .\\ 3. this animal reminds me of my cat that passed away .  \\ 4. I ll never forget this subway .  \\ 5. I miss going to the ocean , the river reminds me of childhood in the country .\end{tabular} \\
%\midrule
%\textbf{Skeptical} & \begin{tabular}[c]{@{}l@{}}1. i doubt that is her child , i dont think they could build that .   \\ 2. i m not sure that those are planes in the air , i doubt she earned it on her own .\\ 3. i don t think the butterfly looks like nice in real life .  \\ 4. did a kid make this ? i am not sure if this meeting is going well for this guy .  \\ 5. are they even playing a song ? i am wondering why this fire started . \end{tabular} \\
\bottomrule
\end{tabular}
\end{table}

\subsection{More Generated Examples}
